# Supplementary material for: Airborne Magnetic Anomaly Navigation with Neural-Network-Augmented Online Calibration
Source: arXiv:2603.08265 source file (2026-03-09)
Supplement: Supplementary file 1 [file finite_differences.tex]

\section{Finite Differences for the Map Matching Jacobian}
\label{app:finite_differences}
\begin{align}
\begin{split}
\frac{\partial \bfh}{\partial \boxi_3} 
&= \frac{\partial \bfh}{\partial \mu} \frac{\partial \mu }{\partial \delta \bfp} \frac{\partial \delta \bfp}{\partial \boxi_3} + \frac{\partial \bfh}{\partial \lambda} \frac{\partial \lambda}{\partial \delta \bfp} \frac{\partial \delta \bfp}{\partial \boxi_3} + \frac{\partial \bfh}{\partial h} \frac{\partial h }{\partial \delta \bfp} \frac{\partial \delta \bfp}{\partial \boxi_3} \\
&= \left( \frac{\partial \bfh}{\partial \mu} \frac{\partial \mu }{\partial \delta \bfp}  + \frac{\partial \bfh}{\partial \lambda} \frac{\partial \lambda}{\partial \delta \bfp}  + \frac{\partial \bfh}{\partial h} \frac{\partial h }{\partial \delta \bfp} \right) \hbfR_{eb}, \\
\end{split}
\end{align}
where the finite differences are obtained as
\begin{align}
\begin{split}
 \frac{\partial \bfh}{\partial \boxi_{3,x}} 
 &= ( \bfh (\mu + \delta \mu_x, \lambda, h) + \bfh(\mu, \lambda + \delta \lambda_x, h) \\ &+ \bfh(\mu, \lambda, h + \delta h_x) - 3 \bfh(\mu, \lambda, h)) \frac{1}{\delta p},
 \end{split}
 \end{align}
 with
 \begin{align*}
 \begin{split}
\delta \mu_x &= \delta p \frac{\partial \mu}{\partial \delta p_x} = \delta p \frac{\mu(p_x + \delta p, p_y, p_z) - \mu(p_x - \delta p, p_y, p_z)}{2 \delta p} \\
\delta \lambda_x & = \delta p \frac{\partial \lambda}{\partial \delta p_x} = \delta p \frac{\lambda(p_x + \delta p, p_y, p_z) - \lambda(p_x - \delta p, p_y, p_z)}{2 \delta p}\\
\delta h_x & = \delta p \frac{\partial h}{\partial \delta p_x} = \delta p \frac{h(p_x + \delta p, p_y, p_z) - h(p_x - \delta p, p_y, p_z)}{2 \delta p}.
\end{split}
\end{align*}
A finite spacing of $\delta p = 10^{-6}$ was chosen. $\frac{\partial \bfh}{\partial \boxi_{3,y}}$ and $\frac{\partial \bfh}{\partial \boxi_{3,z}}$ are calculated analogously.
