# Supplementary material for: Airborne Magnetic Anomaly Navigation with Neural-Network-Augmented Online Calibration
Source: arXiv:2603.08265 source file (2026-03-09)
Supplement: Supplementary file 2 [file pinson_model.tex]

\section{Error-State Model for global inertial navigation in geographical coordinates}
\label{sec:pinson_model}

\todo[inline, color = orange]{Here, the Block matrices of the error state model should be added}
